# Supplementary material for: Graphs of Edge-Intersecting and Non-Splitting One Bend Paths in a Grid
Source: arXiv:1512.06440 source file (2017-06-09)
Supplement: Supplementary file 1 [file appendix.tex]

\section{Unused figures}
\begin{figure}
\commentfig{\includegraphics[width=1.0\textwidth]{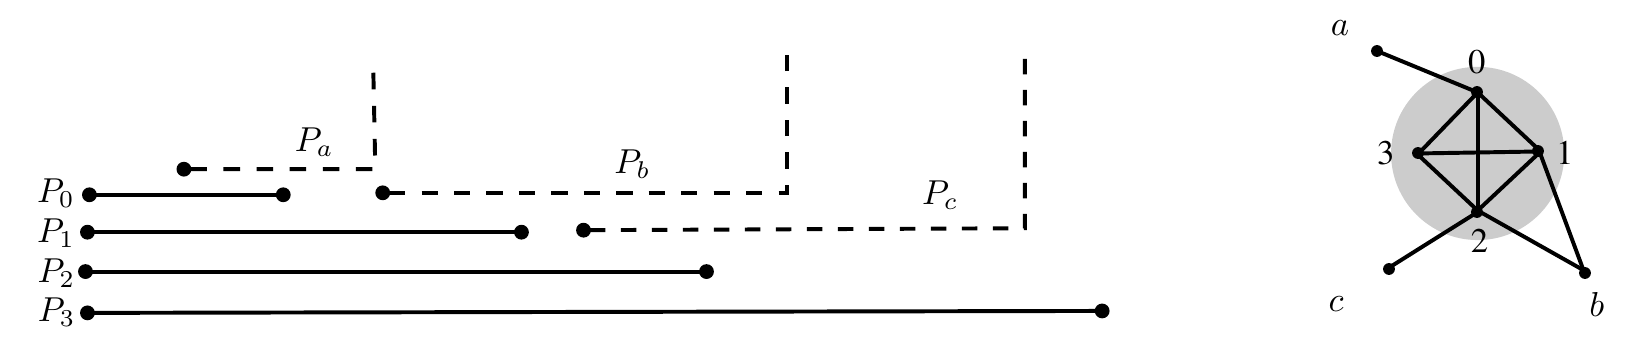}}
\caption{The left side depicts a representation of the $\boneenpg$ split graph on the right.}\label{fig:B1ENPG-split-neighborhoods}
\end{figure}
